# Supplementary material for: Multi-Task Learning with Prior Information
Source: arXiv:2301.01572 source file (2023-01-04)
Supplement: Supplementary file 1 [file appendix.tex]

\section{Appendix}\label{app}
\subsection{Proof of Lemma \ref{lem:1}}
This proof can be found in \cite{beck2009fast}. 
\begin{proof}[Proof of \ref{lem:1}]
	First from the inequality $F(prox_{\eta_P}(\mathbf{P}))
     \leq M_{\mathbf{P},\eta_P}(prox_{\eta_P}(\mathbf{P}))$, we have:
     \begin{equation}\label{eq:inq}
         F(\mathbf{A}) - F(prox_{\eta_P}(\mathbf{P})) \geq F(\mathbf{A}) - M_{\mathbf{P},\eta_P}(prox_{\eta_P}(\mathbf{P})).
     \end{equation}
	Since $F(x) = f(x) + g(x)$ and $f(x), g(x)$ are convex: 
	\begin{equation}\label{eq:fg}
	\begin{aligned}
	    & f(\mathbf{A}) \geq f(\mathbf{P}) + \langle \mathbf{A} - \mathbf{P}, \nabla f(\mathbf{P}) \rangle;\\
	    & g(\mathbf{A}) \geq g(prox_{\eta_P}(\mathbf{P})) + \langle \mathbf{A} - prox_{\eta_P}(\mathbf{P}), \gamma(\mathbf{P}) \rangle,
	\end{aligned}
	\end{equation}
	where $\gamma(\mathbf{P})$ is defined as $\gamma(\mathbf{P}) \in \partial g(prox_{\eta_P}(\mathbf{P}))$ and $\nabla f(\mathbf{P}) + \eta_P(prox_{\eta_P}(\mathbf{P}) - \mathbf{P}) + \gamma(\mathbf{P}) = 0$.
	Summing the inequalities in Eq. (\ref{eq:fg}) yields
	\begin{equation}
     \begin{aligned}
     \label{eq:sum}
	    F(\mathbf{A}) \geq & f(\mathbf{P}) + \langle \mathbf{A} - \mathbf{P}, \nabla f(\mathbf{P}) \rangle + g(prox_{\eta_P}(\mathbf{P})) \\
     & + \langle \mathbf{A} - prox_{\eta_P}(\mathbf{P}), \gamma(\mathbf{P}) \rangle.
     \end{aligned}
	\end{equation}
	And by the definition of $prox_{\eta_P}(\mathbf{P})$, we have
	\begin{equation}\begin{aligned} \label{eq:prox}
	    M_{\mathbf{P},\eta_P}(prox_{\eta_P}(\mathbf{P})) =  & f(\mathbf{P}) + \langle prox_{\eta_P}(\mathbf{P}) - \mathbf{P}, \nabla f(\mathbf{P}) \rangle \\
     & + \frac{\eta_P}{2} \|prox_{\eta_P}(\mathbf{P}) - \mathbf{P} \|^2 + g(prox_{\eta_P}(\mathbf{P})).
	\end{aligned}\end{equation}
	Therefore, plugging in Eq. (\ref{eq:sum}) and Eq. (\ref{eq:prox}) in Eq. (\ref{eq:inq}) gives
	\begin{equation}
	    \begin{aligned}
	        & F(\mathbf{A}) - F(prox_{\eta_P}(\mathbf{P}))\\
          \geq & - \frac{\eta_P}{2} \|prox_{\eta_P}(\mathbf{P}) - \mathbf{P} \|^2 + \langle \mathbf{A} - prox_{\eta_P}(\mathbf{P}), \gamma(\mathbf{P}) +  \nabla f(\mathbf{P}) \rangle \\
	        = & - \frac{\eta_P}{2} \|prox_{\eta_P}(\mathbf{P}) - \mathbf{P} \|^2 + \eta_P \langle \mathbf{A} - prox_{\eta_P}(\mathbf{P}), \mathbf{P} - prox_{\eta_P}(\mathbf{P}) \rangle \\
	         = & \frac{\eta_P}{2} \|prox_{\eta_P}(\mathbf{P}) - \mathbf{P} \|^2 + \eta_P \langle \mathbf{P} - \mathbf{A}, prox_{\eta_P}(\mathbf{P}) - \mathbf{P}  \rangle.
	    \end{aligned}
	\end{equation}
\end{proof}

\subsection{Proof of Theorem \ref{thm:ista}}
The following proof is modified based on \cite{beck2009fast}. 
\begin{proof}[Proof of \ref{thm:ista}]
Invoking Lemma \ref{lem:1} with $\mathbf{A} = \mathbf{P}^*, \mathbf{P} = \mathbf{P}_n,$ and $\eta_P = \eta_{n+1}$, we have:
\begin{equation}\label{eq:4.2.1}
    \begin{aligned}
    &\frac{2}{\eta_{n+1}} F(\mathbf{P}^*) - F(\mathbf{P}_{n+1}) \\
     \geq & \|\mathbf{P}_{n+1} - \mathbf{P}_n \|^2 + 2 \langle \mathbf{P}_n - \mathbf{P}^*,  \mathbf{P}_{n+1} - \mathbf{P}_n \rangle \\
     =  & \|\mathbf{P}^* -  \mathbf{P}_{n+1}\|^2 - \|\mathbf{P}^* -  \mathbf{P}_{n}\|^2,
    \end{aligned}
\end{equation}
and we have the fact that 
\begin{equation}\label{eq:4.2.2}
    \alpha L_P \leq \eta_k \leq \beta L_P,
\end{equation}
where $L_P$ is the Lipschitz constant of $f(\mathbf{P})$ regarding to $\mathbf{P}$, $\beta$ is the $\beta_P$ initialized in \Cref{alg:2}, $\alpha = \min \frac{\eta_{1,2, \dots, k}}{L_P}$. 
Combine Eq. (\ref{eq:4.2.1}) and Eq. (\ref{eq:4.2.2}), and because $F(\mathbf{P}^*) \leq F(\mathbf{P}_{n+1})$, we have:
\begin{equation}
    \frac{2}{\beta L_P} F(\mathbf{P}^*) - F(\mathbf{P}_{n+1}) 
     \geq \|\mathbf{P}^* -  \mathbf{P}_{n+1}\|^2 - \|\mathbf{P}^* -  \mathbf{P}_{n}\|^2.
\end{equation}
Summing the above inequality over $n = 0, 1, \dots, k-1$ gives
\begin{equation}\label{eq:4.2.3}
    \frac{2}{\beta L_P} (kF(\mathbf{P}^*) - \sum_{n=0}^{k-1}F(\mathbf{P}_{n+1}) 
     \geq \|\mathbf{P}^* -  \mathbf{P}_{k}\|^2 - \|\mathbf{P}^* -  \mathbf{P}_{0}\|^2.
\end{equation}
Similarly, invoking Lemma \ref{lem:1} again with $\mathbf{A} = \mathbf{P} = \mathbf{P}_n$, and $\eta_P = \eta_{n+1}$, we get
\begin{equation}
    \begin{aligned}
    \frac{2}{\eta_{n+1}} F(\mathbf{P}_n) - F(\mathbf{P}_{n+1}) 
    & \geq \|\mathbf{P}_{n+1} - \mathbf{P}_n \|^2,
    \end{aligned}
\end{equation}
since $\eta_{n+1} \geq \alpha L_P$ and $F(\mathbf{P}_n) \leq F(\mathbf{P}_{n+1})$, it follows that
\begin{equation}\label{eq:4.2.4}
    \frac{2}{\alpha L_P} F(\mathbf{P}_n) - F(\mathbf{P}_{n+1}) 
     \geq \|\mathbf{P}_n -  \mathbf{P}_{n+1}\|^2.
\end{equation}
Multiplying Eq. (\ref{eq:4.2.4}) by n and summing over $n = 0, 1, \dots, k-1$ gives
\begin{equation}\label{eq:4.2.5}
    \frac{2}{\alpha L_P} (-kF(\mathbf{P}_k)) + \sum_{n=0}^{k-1}F(\mathbf{P}_{n+1}))
     \geq \sum_{n=0}^{k-1} n\|\mathbf{P}_n -  \mathbf{P}_{n+1}\|^2.
\end{equation}
Adding Eq. (\ref{eq:4.2.3}) and Eq. (\ref{eq:4.2.5}) times $\alpha / \beta$, we obtain
\begin{equation}\begin{aligned}\label{eq:4.2.6}
    & \frac{2k}{\beta L_P} (F(\mathbf{P}^*)) - F(\mathbf{P}_{k}))\\
     \geq & \|\mathbf{P}^* -  \mathbf{P}_{k}\|^2 + \frac{\alpha}{\beta} \sum_{n=0}^{k-1} n\|\mathbf{P}_n -  \mathbf{P}_{n+1}\|^2 - \|\mathbf{P}^* -  \mathbf{P}_{0}\|^2.
\end{aligned}\end{equation}
Therefore it follows the following inequality:
\begin{equation}
 F(\mathbf{P}_{k}) - F(\mathbf{P}^*)) \leq \frac{\beta L_P  \|\mathbf{P}^* -  \mathbf{P}_{0}\|^2}{2k}.
\end{equation}
\end{proof}
